# Supplementary material for: RecoveryChaining: Learning Local Recovery Policies for Robust Manipulation
Source: arXiv:2410.13979 source file (2025-03-07)
Supplement: Supplementary file 1 [file 8_appendix.tex]

\begin{appendices}
% \appendix
% \section{Ablation Study}
\section{Effect of Offline Data on Skill Chaining}
We study the effect of the size of offline data on the quality of recovery learning using skill chaining.
To do so, we collect datasets A, B and C consisting of 250, 400 and 600 nominal trajectories, learn the preconditions and then train recovery policies in the \textsc{PickPlace} task.
The learning curves of the recovery policies and the actual recovery rates are plotted in figure~\ref{fig:sc_ablation}.
The recovery policy with the largest dataset C performs better than others initially but degrades with further training.
Overall, we find that recovery learning with learned reward models converges faster (in 100k timesteps) but to a highly sub-optimal policy which does not improve with further training.
% We postulate two reasons for this:
% \begin{enumerate}
    % \item Despite being bigger, datasets B and C are not that different from A because they were generated by rolling out the nominal controllers.
    % \item Performance on dataset C degrades with further training probably because the RL policy diverged too much from the nominal dataset and hence received incorrect reward signals.
% \end{enumerate}

\begin{figure}[th]
    \centering
    \begin{subfigure}{1.0\columnwidth}
    \includegraphics[width=1.0\columnwidth]{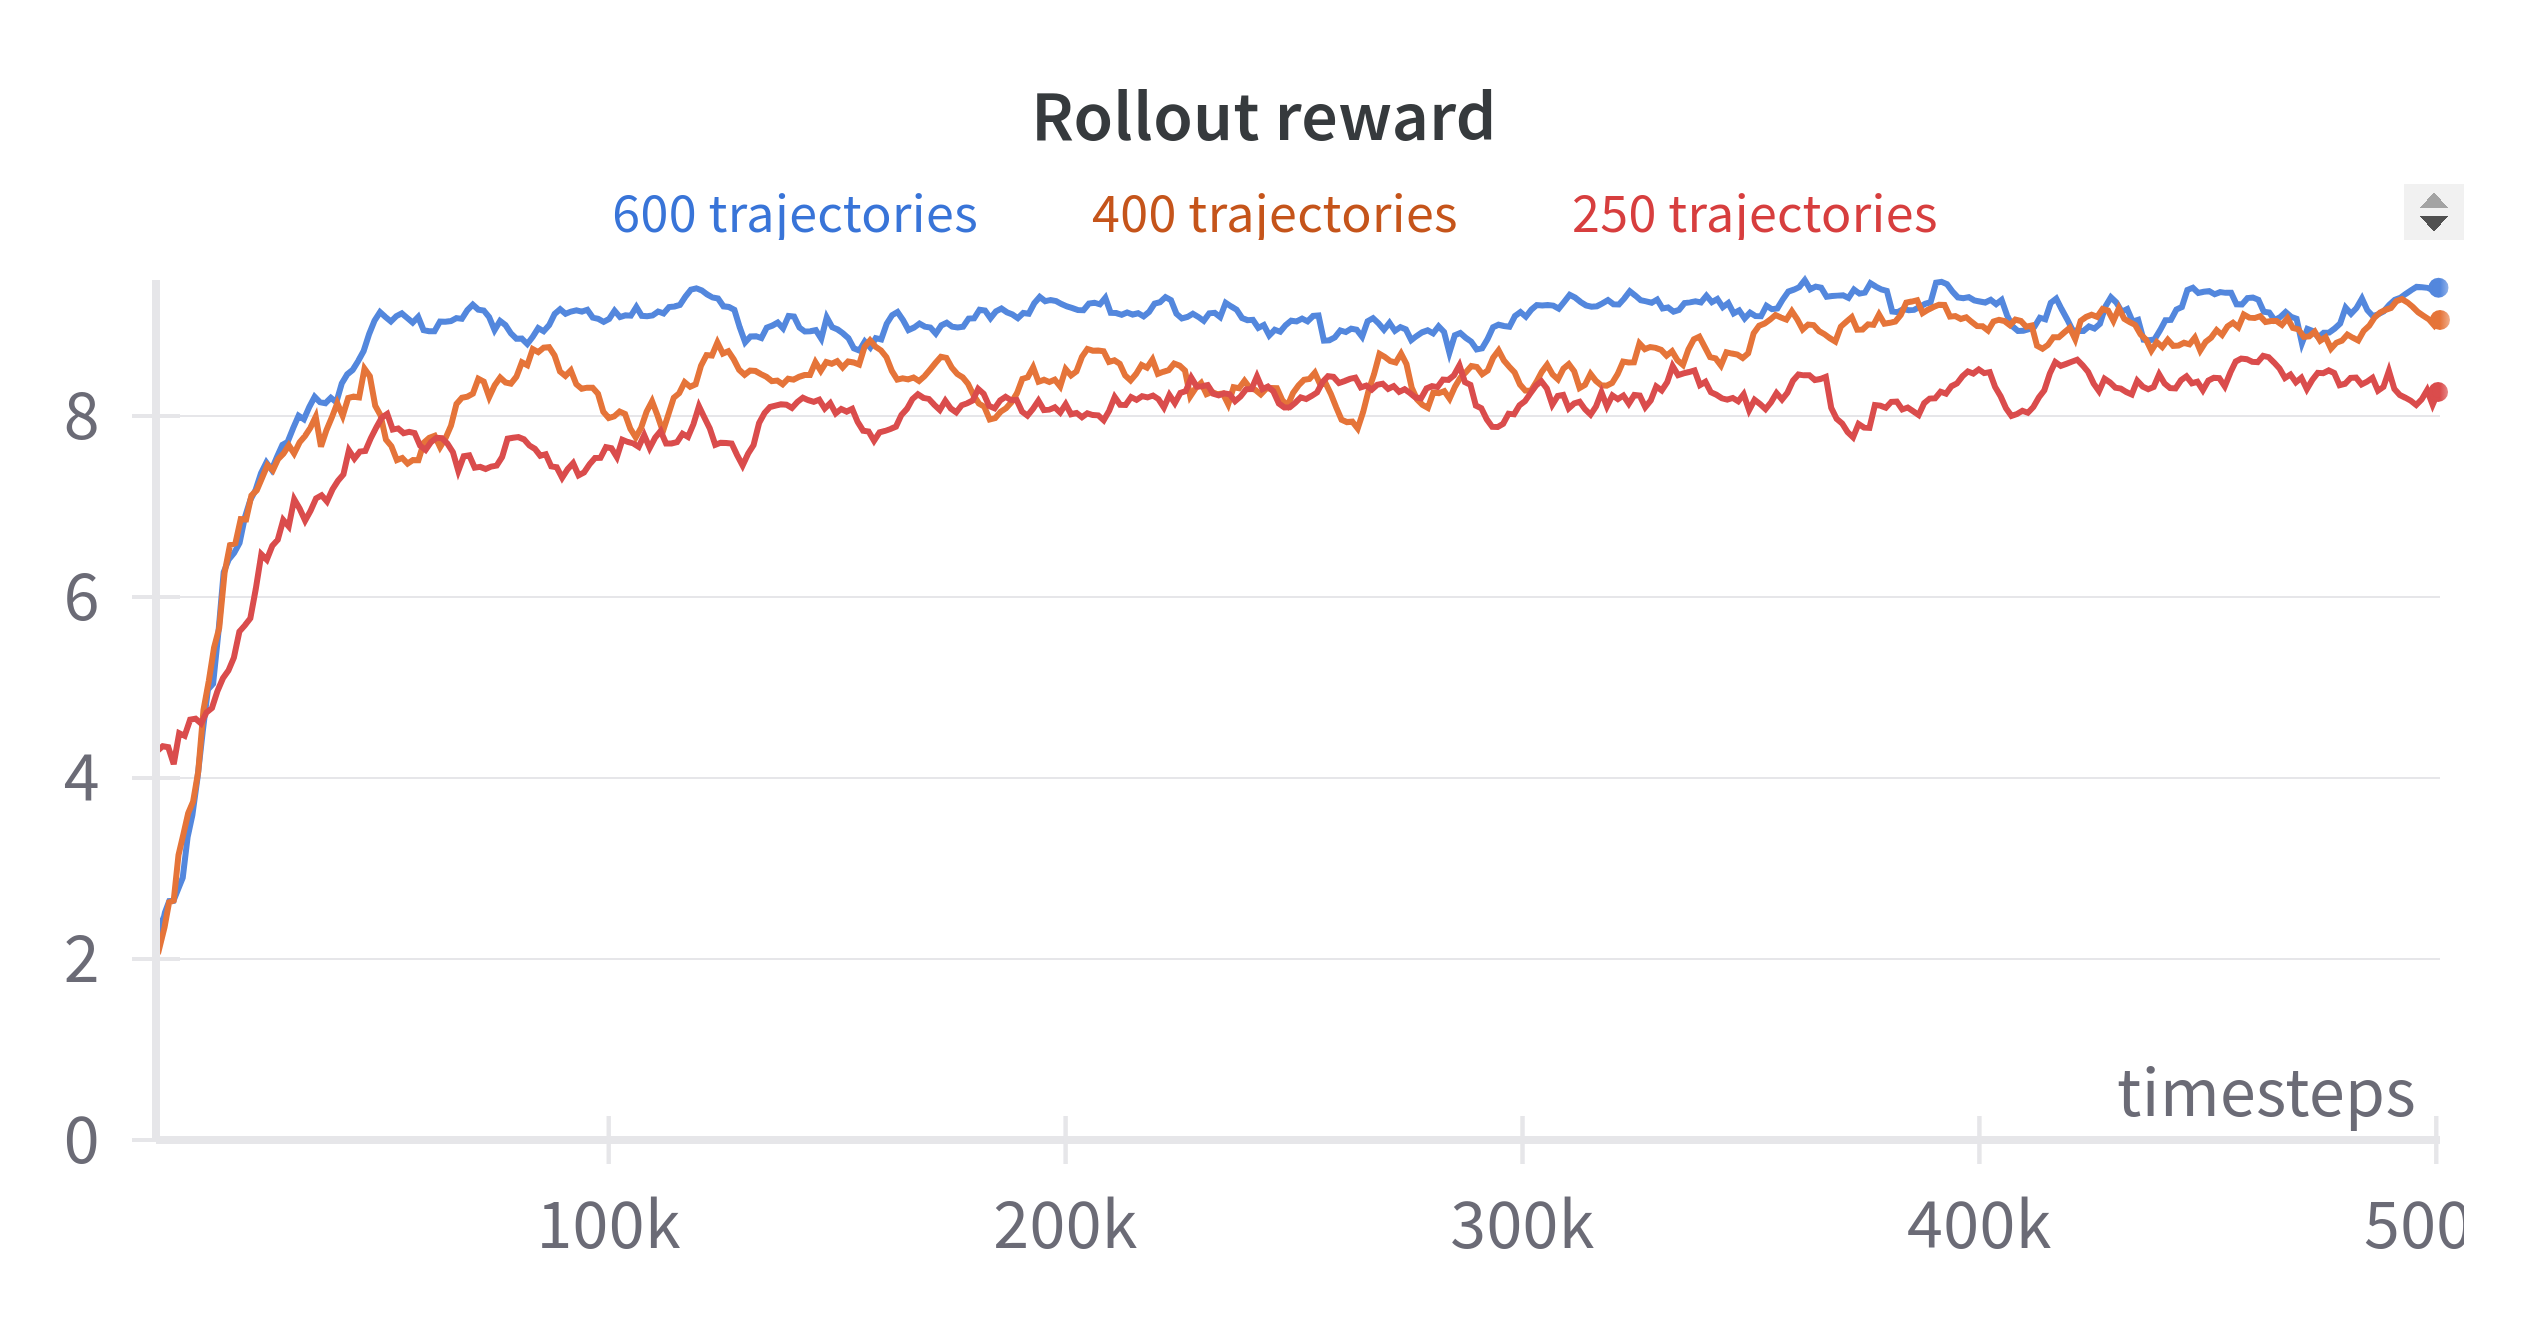}
    \caption{Learning curves of skill chaining with different datasets on \textsc{PickPlace} task.
    The agent with 600 trajectories achieves marginally better final reward than the other agents.}
    \end{subfigure}
    \begin{subfigure}{1.0\columnwidth}
    \includegraphics[width=1.0\columnwidth]{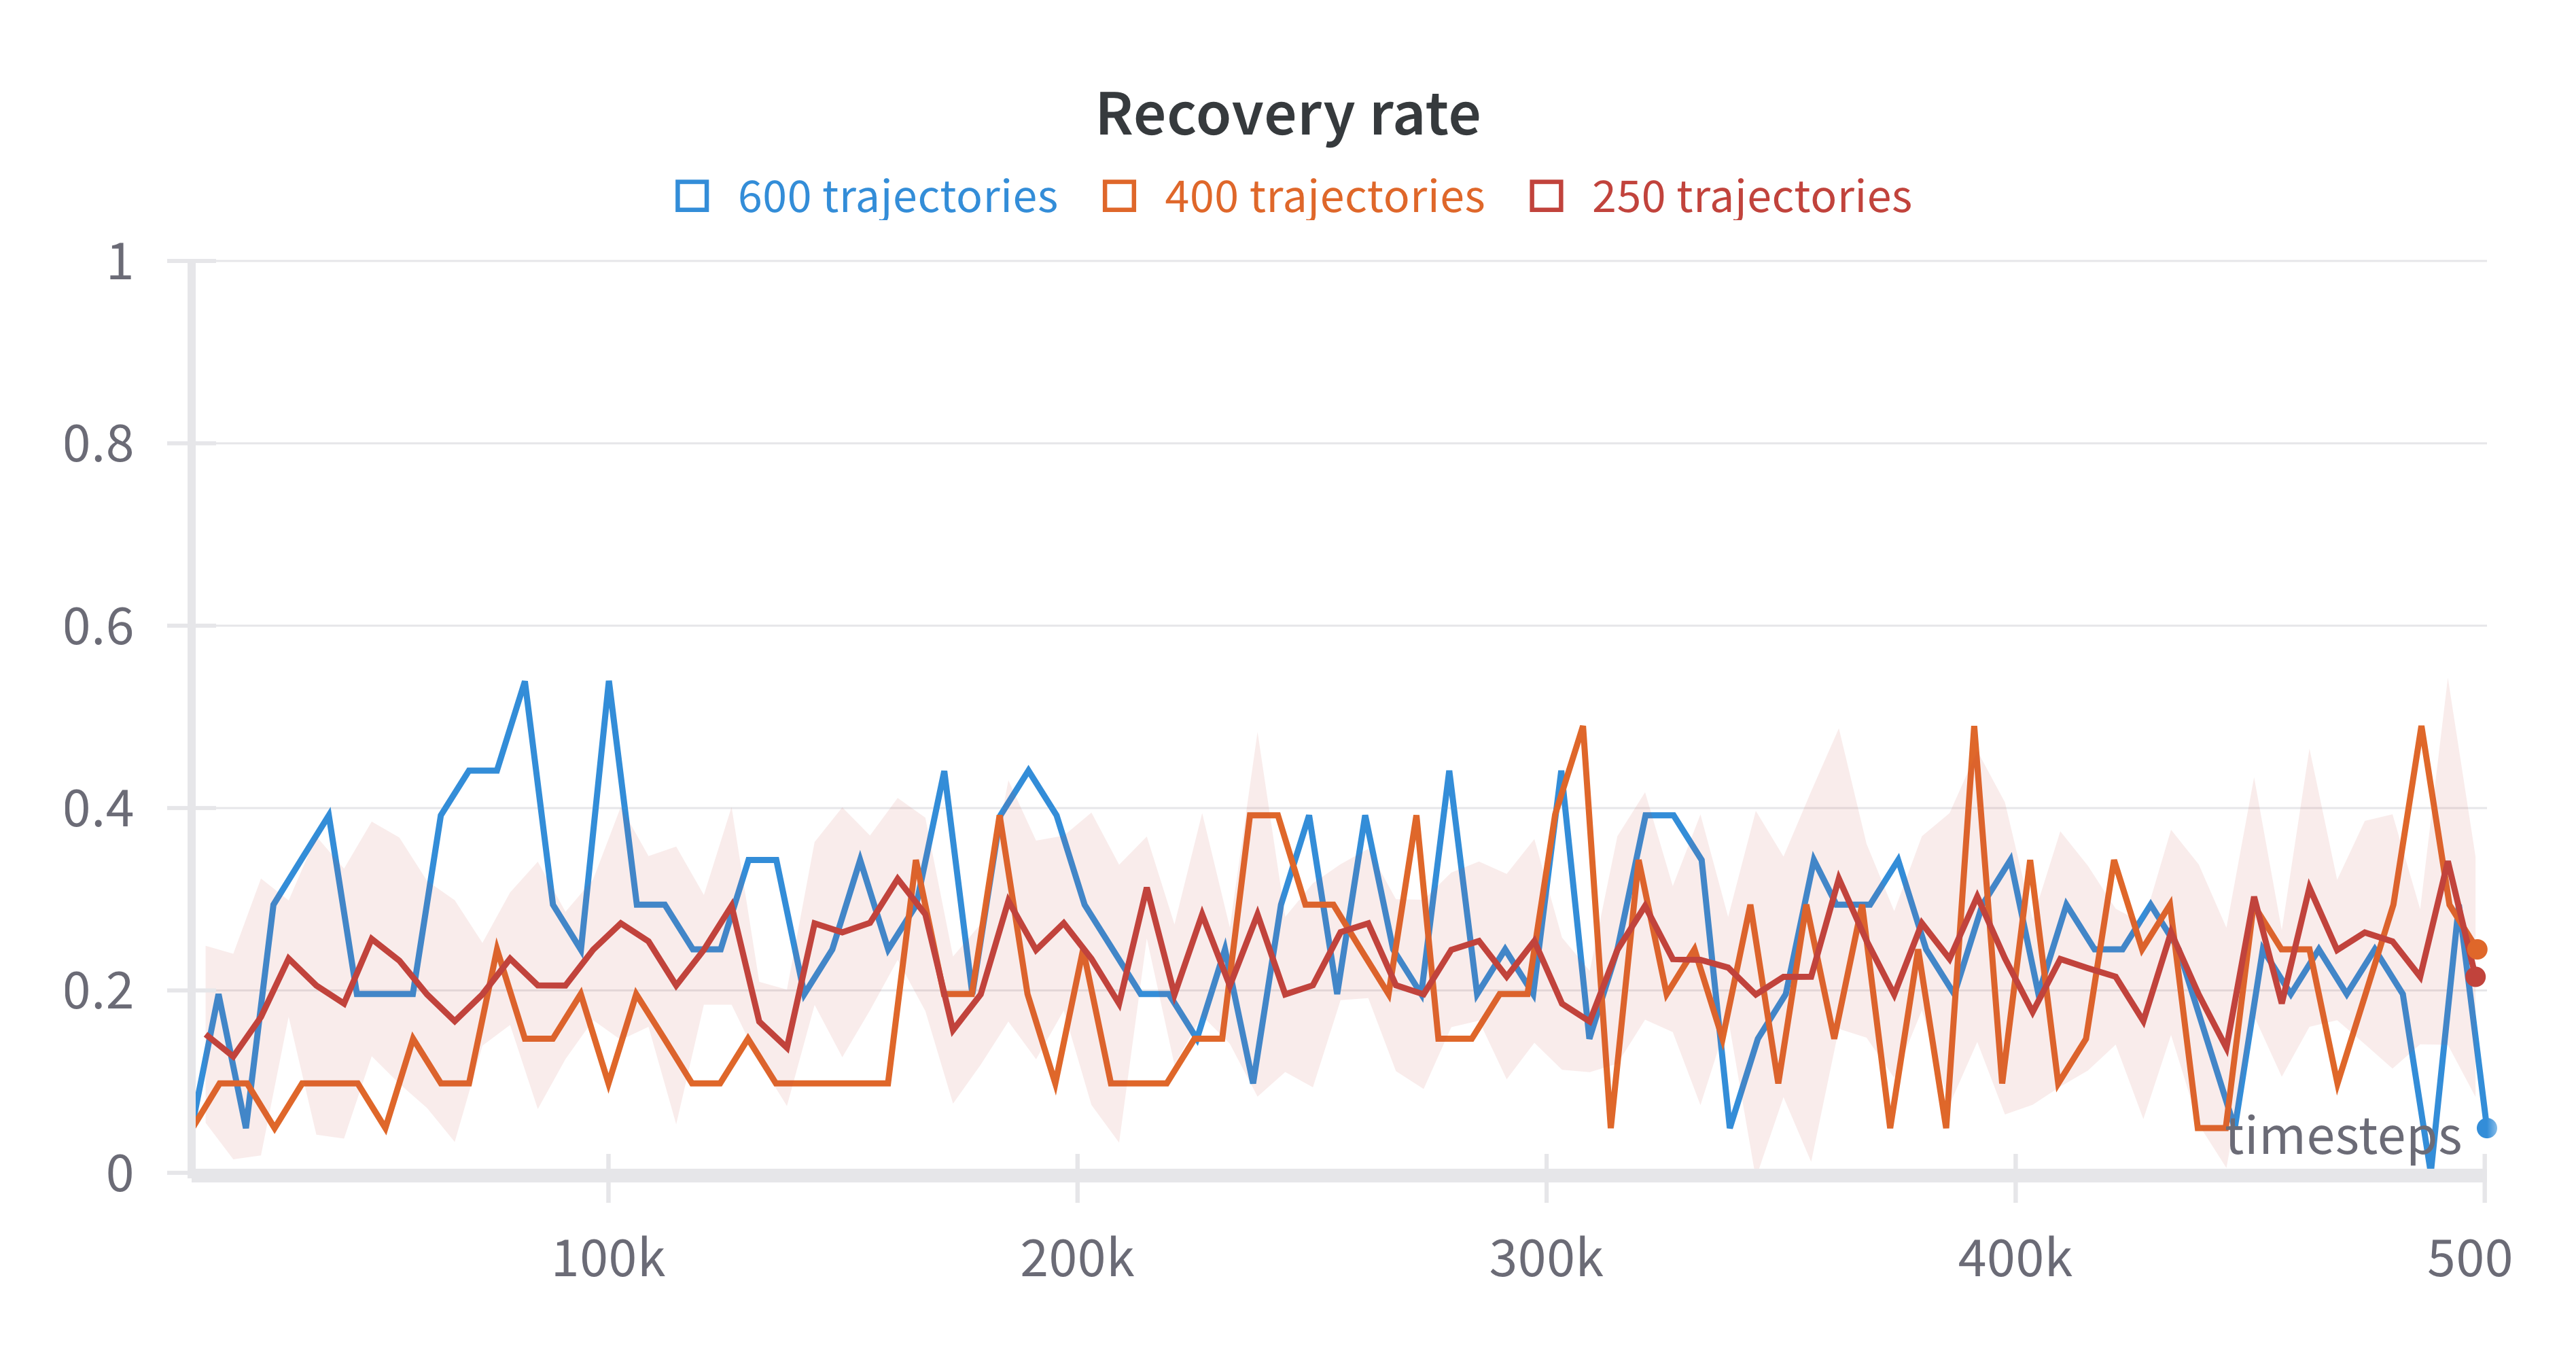}
    \caption{Actual recovery rate of the policies being learned.
    We do not observe any significant and stable improvement in recovery rate from training the preconditions using a larger dataset.
    % of nominal trajectories does not have a consistent and stable effect on the performance of the recovery policy.
    }
    \end{subfigure}
    \caption{}
    \label{fig:sc_ablation}
\end{figure}

% \subsection{Should the Switch Action Be Terminal?}

% \subsection{Residual RL}

% \section{Discussion}
% \subsection{Markovian vs Non-Markovian Nominal Controllers}

\section{Additional Experimental Details}
\textbf{Action Space.} We use just translation action primitives for the \textsc{Shelf} task and translation + rotation action primitives for the \textsc{PickPlace} task.

\textbf{Reward.} We use a sparse reward function wherein the agent receives a reward of 1 on achieving the goal and 0 otherwise in all our domains.

\begin{table}[bh]
\centering
\begin{tabular}{ll}
\toprule
\textbf{PPO Parameter} & \textbf{Value} \\
\midrule\\
rollout steps      & 120  \\
batch size    & 60   \\
learning rate & 3e-4 \\
hidden units & [256, 256] \\
entropy coefficient & 0 \\
total timesteps & 500k \\
discount & 0.99 \\
\bottomrule
\end{tabular}
\label{tab:hyper}
\end{table}
We use the same set of hyperparameters with PPO in all our experiments.

% \subsection{Pick-Place}
% \subsection{Reinforcement Learning Baseline}

% \section{Shelf}
% \subsection{Reinforcement Learning Baseline}

% While our method is capable of learning recoveries for chained skills, it can also be used to robustify single skills.

\rebuttal{\section{Visualization of Initiation Sets}}
\rebuttal{We visualize the initiation sets of the \textsc{Pick} skill in the pick-place task and the \textsc{Place} skill in the shelf task in figure~\ref{fig:init_sets}.
}

\rebuttal{
\textbf{Pick-place.} We visualize the initiation set of the \textsc{Pick} skill and failures by plotting the $x$ and $y$ positions of the end-effector at those states.
 Most failures occur when the end-effector collides with the top and bottom walls of the bin during pick-up.
 Hence, the failures are concentrated near the top and bottom of the plot.
 The rest of the bin is inside the initiation set of the \textsc{Pick} skill.
 }

\rebuttal{
\textbf{Shelf.} We visualize the initiation set of the \textsc{Place} skill and failures on a side-view of the shelf with origin at the goal.
The goal location, marked with a star, shows the target $y$ and $z$ position of the centroid of the box.
The box collides with the bottom of the shelf if its centroid is too low, i.e., $z_{box} < z_{goal}$.
}

\begin{figure*}[th]
    \centering
    \includegraphics[width=0.9\columnwidth]{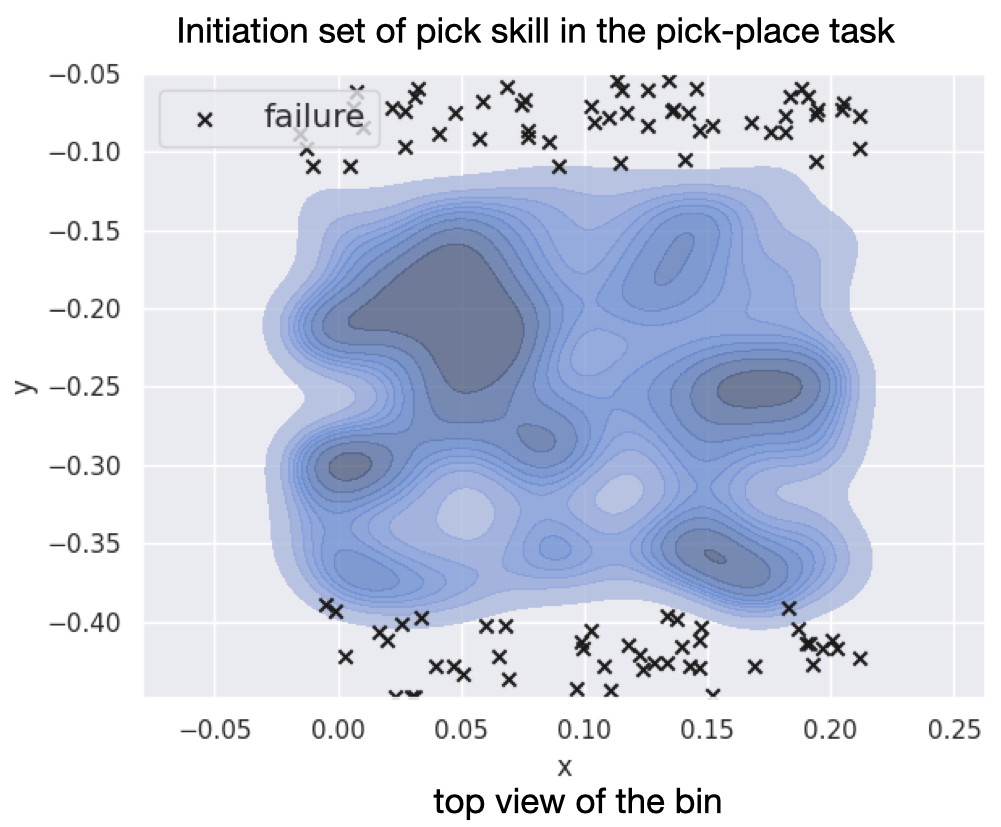}
    \includegraphics[width=0.9\columnwidth]{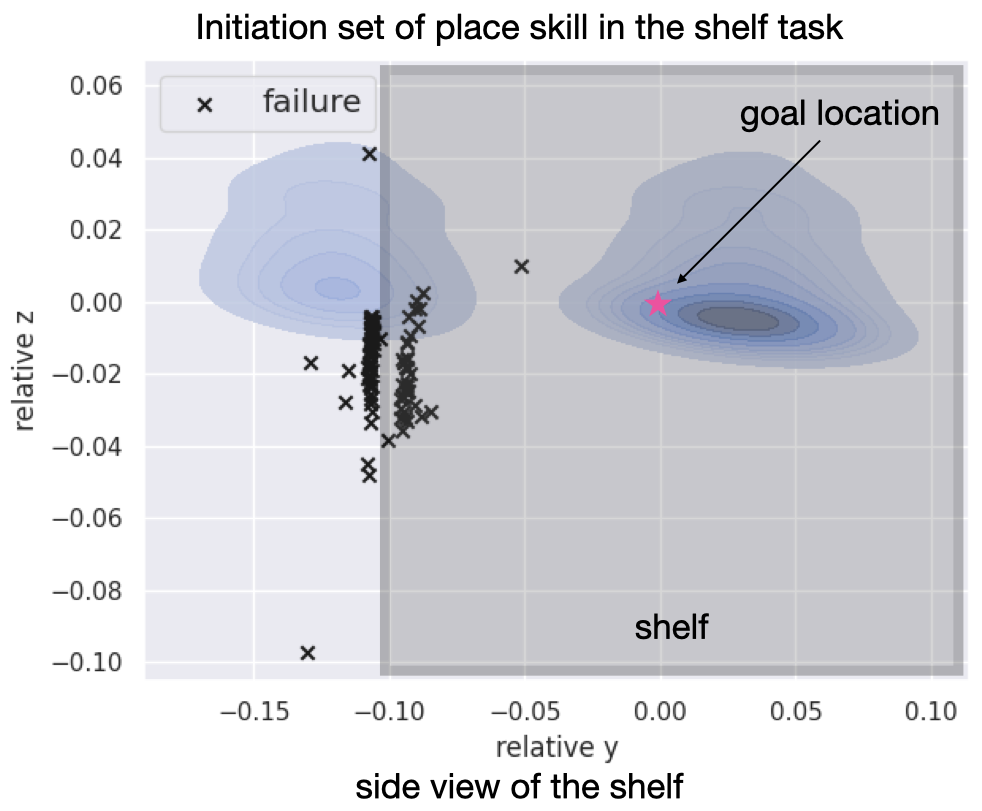}
    \caption{\rebuttal{(left) Initiation set of the \textsc{Pick} skill along with the detected failures in the pick-place task.
    We visualize the $x$ and $y$ positions of the end-effector.
    All the failures are concentrated near the top and bottom walls of the bin due to collision of the end-effector with the walls.
    (right) Initiation set of the \textsc{Place} skill in the shelf task.
    We visualize the relative $y$ and $z$ positions of the box with respect to the target position on the shelf.
    Most of the failures occur due to the collision of the box with the bottom of the shelf.
    Hence, the failures are concentrated around $(-0.1, 0)$.
    }
    }
    \label{fig:init_sets}
\end{figure*}
\end{appendices}
